# Supplementary material for: Entropy-driven liquid-liquid separation in supercooled water
Source: arXiv:1207.2101 ancillary file (2017-08-11)
Supplement: Supplementary file 1 [file HoltenAnisimov2012Supplement.pdf]

# Entropy-driven liquid–liquid separation in supercooled water – Supplement

V. Holten and M. A. Anisimov
*Institute for Physical Science and Technology and Department of Chemical and Biomolecular Engineering, University of Maryland, College Park, Maryland 20742, USA*

(Dated: 9 July 2012)

## 1. TWO-STATE THERMODYNAMICS FOR SUPERCOOLED WATER

It is convenient to introduce dimensionless variables,

$$\hat{T} = \frac{T}{T_c}, \quad \hat{P} = \frac{PV_c}{k_B T_c}, \quad \hat{G} = \frac{G}{k_B T_c},$$
$$\Delta\hat{T} = \frac{T - T_c}{T_c}, \quad \Delta\hat{P} = \frac{(P - P_c)V_c}{k_B T_c},$$

and rewrite equation (2) for the Gibbs energy of liquid water as

$$\frac{\hat{G}}{\hat{T}} = \frac{\hat{G}^A}{\hat{T}} + x\ln K + x\ln x + (1-x)\ln(1-x) + \omega x(1-x). \tag{S1}$$

In the theory of phase transitions, critical behaviour is described by two independent scaling fields, the ordering field $h_1$ and non-ordering field $h_2$, and a scaling field $h_3$ that depends on $h_1$ and $h_2$ and serves as the critical part of a field-dependent thermodynamic potential. Two scaling densities, a strongly fluctuating order parameter $\phi_1$ and a weakly fluctuating scaling density $\phi_2$, are conjugate to the scaling fields, such that

$$dh_3 = \phi_1\, dh_1 + \phi_2\, dh_2. \tag{S2}$$

As shown by Bertrand and Anisimov,[1] the athermal-solution model given by equation (S1) corresponds to a specific mapping of scaling fields to physical fields. For the liquid–liquid transition in water near the LLCP, the order parameter is associated with the entropy, contrary to the usual vapour–liquid critical point where it is associated with the density.[2–4] For our two-state model, the scaling fields can be mapped to the physical fields as

$$\begin{aligned} h_1 &= -\ln K = -\frac{\hat{G}^{BA}}{\hat{T}}, \\ h_2 &= -\Delta\hat{P}, \\ h_3 &= -\frac{2(\hat{G}-\hat{G}^A) - \hat{G}^{BA}}{\hat{T}} + \frac{\omega_0}{2}\Delta\hat{P}, \end{aligned} \tag{S3}$$

as illustrated in Fig. S1. In our model, the non-ordering field $h_2$ is associated with the pressure, contrary to the vapour–liquid critical point, where it is associated with the temperature and thus called the 'thermal field'. The field $h_3$, the critical part of the thermodynamic potential, is related to $\hat{G}/\hat{T}$ in such a way that at the critical point

$$\phi_1 = \left(\frac{\partial h_3}{\partial h_1}\right)_{h_2} = 0 \quad \text{and} \quad \phi_2 = \left(\frac{\partial h_3}{\partial h_2}\right)_{h_1} = 0. \tag{S4}$$

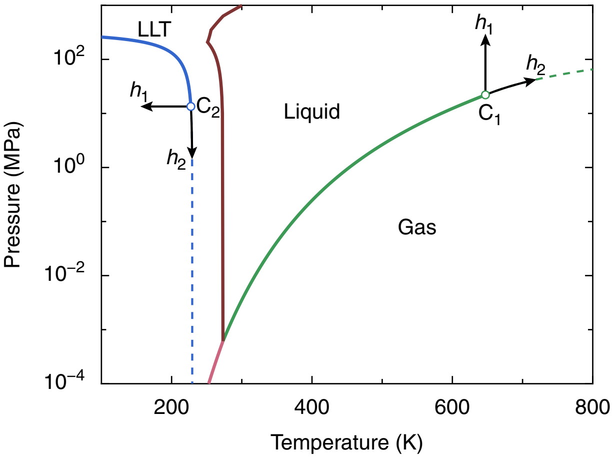


FIG. S1. **Scaling fields for the liquid–liquid and liquid–vapour criticality.** The liquid–liquid transition LLT (blue) ends at the critical point $C_2$. The arrows indicate the directions of the ordering field $h_1$ and non-ordering field $h_2$. The green curve is the liquid–vapour transition, which ends at critical point $C_1$. Dashed lines are the corresponding Widom lines. The melting curve is shown in brown and the sublimation curve in pink.

Specifically, for this mapping, the order parameter $\phi_1$ is related to the concentration $x = x_e$ as

$$\phi_1 = \Delta\hat{x} \equiv (x - x_c)/x_c, \tag{S5}$$

where the critical concentration $x_c = 1/2$. Close to the critical point, the behaviour of the two-state model given by equation (S1) can be described with mean-field Landau theory.[5] To enable a comparison between the model and Landau theory, we transform the field-dependent potential $\hat{G}(\hat{T},\hat{P})/\hat{T}$ to a potential $\Phi(\phi_1, h_2)$, which in our model appears to be the Gibbs energy of mixing, by means of a Legendre transform,

$$\begin{aligned} \Phi &= -(h_3 - h_1\phi_1) \\ &= 2\left[x\ln x + (1-x)\ln(1-x) + \omega x(1-x) - \frac{\omega_0}{4}\Delta\hat{P}\right]. \end{aligned} \tag{S6}$$

The truncated expansion of the potential $\Phi$ around the critical point in powers of $\Delta\hat{x}$ and $\Delta\hat{P}$ is

$$\Phi \simeq -\frac{1}{2}\omega_0\Delta\hat{P}(\Delta\hat{x})^2 + \frac{1}{6}(\Delta\hat{x})^4.$$

A comparison with the mean-field Landau expansion,[3–5]

$$\Phi \simeq \frac{1}{2}a_0 h_2\phi_1^2 + \frac{1}{4!}u_0\phi_1^4$$

where $a_0$ and $u_0$ are system-dependent amplitudes, shows that for our two-state model $a_0 = \omega_0$ and $u_0 = 4$.

## 2. CALCULATION OF PROPERTIES

All thermodynamic properties can be calculated as derivatives of the Gibbs energy. From equations (S2)–(S3), we derive for the volume and entropy

$$\hat{V} = \left(\frac{\partial \hat{G}}{\partial \hat{P}}\right)_T = \frac{\hat{T}}{2}\left[\phi_2 + \frac{\omega_0}{2} + L_{\hat{P}}(\phi_1 + 1)\right] + \hat{V}^{\mathrm{A}},$$
$$\hat{S} = -\left(\frac{\partial \hat{G}}{\partial \hat{T}}\right)_P = -\frac{\hat{G} - \hat{G}^{\mathrm{A}}}{\hat{T}} - \frac{1}{2}L_{\hat{T}}\hat{T}(\phi_1 + 1) + \hat{S}^{\mathrm{A}}, \tag{S7}$$

where $\hat{V}^{\mathrm{A}}$ and $\hat{S}^{\mathrm{A}}$ are the volume and entropy of pure A, and

$$L_{\hat{T}} \equiv \left(\frac{\partial \ln K}{\partial \hat{T}}\right)_P = \lambda(1 + b\Delta\hat{P}),$$
$$L_{\hat{P}} \equiv \left(\frac{\partial \ln K}{\partial \hat{P}}\right)_T = \lambda(a + b\Delta\hat{T}).$$

For the response functions, namely, isothermal compressibility $\hat{\kappa}_T$, thermal expansion coefficient $\hat{\alpha}_P$, and isobaric heat capacity $\hat{C}_P$, we find:

$$\hat{\kappa}_T\hat{V} = \frac{\hat{T}}{2}(L_{\hat{P}}^2\chi_1 + 2L_{\hat{P}}\chi_{12} + \chi_2) + \hat{\kappa}_T^{\mathrm{A}}\hat{V}^{\mathrm{A}},$$
$$\hat{\alpha}_P\hat{V} = \frac{L_0 b}{2}\hat{T}(\phi_1 + 1) + \frac{\hat{V} - \hat{V}^{\mathrm{A}}}{\hat{T}} - \frac{\hat{T}L_{\hat{T}}}{2}(L_{\hat{P}}\chi_1 + \chi_{12}) + \hat{\alpha}_P^{\mathrm{A}}\hat{V}^{\mathrm{A}},$$
$$\hat{C}_P = -L_{\hat{T}}\hat{T}(\phi_1 + 1) + \frac{1}{2}L_{\hat{T}}^2\hat{T}^2\chi_1 + \hat{C}_P^{\mathrm{A}}. \tag{S8}$$

where the properties with superscript A are those of pure component A. The heat capacity at constant volume $C_V$ was calculated using the thermodynamic relation[6]

$$C_V = C_P - \frac{T\alpha_P^2}{\rho\kappa_T}. \tag{S9}$$

The strong susceptibility $\chi_1$, the weak susceptibility $\chi_2$, and the cross susceptibility $\chi_{12}$ are defined as

$$\chi_1 = \left(\frac{\partial \phi_1}{\partial h_1}\right)_{h_2}, \qquad \chi_2 = \left(\frac{\partial \phi_2}{\partial h_2}\right)_{h_1},$$
$$\chi_{12} = \left(\frac{\partial \phi_1}{\partial h_2}\right)_{h_1} = \left(\frac{\partial \phi_2}{\partial h_1}\right)_{h_2}.$$

To obtain expressions for the scaling densities and susceptibilities, we return to the potential $\Phi(\phi_1, h_2)$ of equation (S6). The differential of $\Phi$ is

$$\mathrm{d}\Phi = h_1\,\mathrm{d}\phi_1 - \phi_2\,\mathrm{d}h_2.$$

As seen from equation (S7), the entropy after subtracting the entropy background is proportional to the order parameter $\phi_1$. The weakly fluctuating scaling density is

$$\phi_2 = -\left(\frac{\partial \Phi}{\partial h_2}\right)_{\phi_1} = \left(\frac{\partial \Phi}{\partial \hat{P}}\right)_x = -\frac{\omega_0}{2}(\Delta\hat{x})^2. \tag{S10}$$

The scaling susceptibilities are

$$\chi_1^{-1} = \left(\frac{\partial^2 \Phi}{\partial \phi_1^2}\right)_{h_2} = \frac{1}{4}\left(\frac{\partial^2 \Phi}{\partial x^2}\right)_{\hat{P}} = \frac{1}{2x(1-x)} - \omega. \tag{S11}$$
$$\chi_{12} = -\left(\frac{\partial^2 \Phi}{\partial \phi_1 \partial h_2}\right)\chi_1 = \frac{1}{2}\left(\frac{\partial^2 \Phi}{\partial x \partial \hat{P}}\right)\chi_1 = -\omega_0\chi_1\Delta\hat{x}.$$
$$\chi_2 = \frac{\chi_{12}^2}{\chi_1} - \left(\frac{\partial^2 \Phi}{\partial h_2^2}\right)_{\phi_1} = \omega_0^2\chi_1(\Delta\hat{x})^2.$$

The procedure to calculate the properties at a certain temperature and pressure is as follows. First, the equilibrium fraction $x_e$ is calculated from equation (3). Then, the scaling densities and susceptibilities are found from equations (S5), (S10), and (S11). Finally, the properties are calculated from equations (S7) and (S8).

## 3. CROSSOVER PROCEDURE

Fluctuations of the order parameter diverge at the critical point and significantly alter the mean-field equation of state in the immediate vicinity of the critical point.[2–5] In scaling theory of critical phenomena, the thermodynamic potential $h_3$ is a homogeneous function of $h_1$ and $h_2$. Asymptotically:

$$h_3 = |h_2|^{2-\alpha} f^{\pm}\left(\frac{h_1}{|h_2|^{2-\alpha-\beta}}\right), \tag{S12}$$

where $f^{\pm}$ is a scaling function and the superscript $\pm$ refers to $h_2 > 0$ and $h_2 < 0$, respectively. The form of the scaling function is universal; however, it contains two thermodynamically independent (but system-dependent) amplitudes which are related to all other asymptotic amplitudes by universal relations. The critical exponents $\alpha$ and $\beta$ are universal within the Ising model/lattice gas class of critical-point universality. We assume that the LLCP in supercooled water belongs, like critical points of all other fluids, to the Ising model/lattice gas universality class.

For $h_1 = 0$ and $h_2 > 0$, there is a single phase characterized by $\phi_1 = 0$ and

$$\phi_2 = \left(\frac{\partial h_3}{\partial h_1}\right)_{h_1} = \frac{A_0^+}{1-\alpha}|h_2|^{1-\alpha}. \tag{S13}$$

For $h_1 = 0$ and $h_2 < 0$, there are two coexisting phases with

$$\phi_1 = \left(\frac{\partial h_3}{\partial h_1}\right)_{h_2} = \pm B_0|h_2|^{\beta}, \tag{S14}$$

and

$$\phi_2 = -\frac{A_0^-}{1-\alpha}|h_2|^{1-\alpha}. \tag{S15}$$

While the superscript $\pm$ refers to the states at $h_2 > 0$ and $h_2 < 0$, the prefactor $\pm$ in equation (S14) refers to the branches of the order parameter on the $h_1 > 0$ and $h_1 < 0$ sides, respectively. In the above expressions $A_0^{\pm}$ and $B_0$ are non-universal amplitudes. The scaling susceptibilities, asymptotically and in zero ordering field, $h_1 = 0$:

$$\chi_1 = \hat{\Gamma}_0^{\pm} |h_2|^{-\gamma} , \tag{S16}$$

$$\chi_2 = \hat{A}_0^{\pm} |h_2|^{-\alpha} , \tag{S17}$$

$$\chi_{12} = -\beta \hat{B}_0 |h_2|^{\beta-1} \ (h_2 < 0) , \ \chi_{12} = 0 \ (h_2 > 0) , \tag{S18}$$

where the critical exponent $\gamma = 2 - \alpha - 2\beta$ and the Ising critical amplitude $\hat{\Gamma}_0^{\pm}$ is related to $\hat{B}_0$ and $\hat{A}_0^{\pm}$ through the universal ratios, $\alpha \hat{\Gamma}_0^{+} \hat{A}_0^{+} / \hat{B}_0^2 \simeq 0.0581$, $\hat{\Gamma}_0^{+}/\hat{\Gamma}_0^{-} \simeq 4.8$, and $\hat{A}_0^{+}/\hat{A}_0^{-} \simeq 0.523$.[7]

To implement a crossover between the asymptotic scaling behaviour and mean-field behaviour given by equation (S1), we will renormalize the potential $\Phi$. This renormalization is carried out by replacing the variables $\Delta \hat{P}$ and $\Delta \hat{x}$ by the variables $\Delta \hat{P}_\times$ and $\Delta \hat{x}_\times$, defined as[3,8]

$$\Delta \hat{P}_\times = \Delta \hat{P} \, \mathcal{T} \mathcal{U}^{-1/2},$$
$$\Delta \hat{x}_\times = \Delta \hat{x} \, \mathcal{D}^{1/2} \mathcal{U}^{1/4},$$

where the rescaling functions $\mathcal{T}$, $\mathcal{U}$, and $\mathcal{D}$ will be defined below. In addition, a kernel term $k$,

$$k = -\frac{1}{2} h_2^2 \mathcal{K},$$

responsible for the singularity in the weak susceptibility $\chi_2$, is added to the potential $\Phi$.[3,4] Here $\mathcal{K}$ is another rescaling function, defined below. The renormalized potential $\Phi_\times$ becomes

$$\begin{aligned} \Phi_\times = \ & 2\big[x_\times \ln x_\times + (1 - x_\times) \ln(1 - x_\times) \\ & + \omega(\Delta \hat{P}_\times) x_\times (1 - x_\times) - \frac{\omega_0}{4} \Delta \hat{P}_\times \big] - \frac{1}{2} (\Delta \hat{P})^2 \mathcal{K}, \end{aligned}$$

where $x_\times = \frac{1}{2}(\Delta \hat{x}_\times + 1)$. Performing a Legendre transform, we find for the renormalized Gibbs energy $\hat{G}_\times$

$$\begin{aligned} \frac{\hat{G}_\times}{\hat{T}} = \ & \frac{\hat{G}^{\mathrm{A}}}{\hat{T}} + x \ln K + x_\times \ln x_\times + (1 - x_\times) \ln(1 - x_\times) \\ & + \frac{1}{4} \omega(\Delta \hat{P}) - \Big(x_\times - \frac{1}{2}\Big)^2 \omega(\Delta \hat{P}_\times) - \frac{1}{4} (\Delta \hat{P})^2 \mathcal{K}. \end{aligned} \tag{S19}$$

The rescaling functions are defined as

$$\mathcal{T} = Y^{(2\nu - 1)/\Delta}, \qquad \mathcal{U} = Y^{\nu/\Delta},$$
$$\mathcal{D} = Y^{(\gamma - 2\nu)/\Delta}, \qquad \mathcal{K} = \frac{c_t^2 \nu}{\alpha \bar{u} \Lambda} (Y^{-\alpha/\Delta} - 1),$$

where $\Delta$ is the so-called Wegner's exponent.[3,4] We adopt the following values of the critical exponents, which correspond to the best theoretical estimates[2,9] and experimental findings:[3,4,10]

$$\nu = 0.630, \qquad \Delta = 0.5,$$
$$\gamma = 1.237, \qquad \alpha = 0.110.$$

The constant $c_t$ is defined as[3]

$$c_t = \frac{a_0}{c_\rho^2}, \qquad c_\rho = \left(\frac{u_0}{u^* \bar{u} \Lambda}\right)^{1/4},$$

where the mean-field amplitudes are $a_0 = \omega_0$ and $u_0 = 4$, the fixed-point coupling constant of renormalization group theory $u^* \simeq 0.472$, and $\bar{u}$ and the molecular cutoff $\Lambda$ are two crossover parameters. The crossover function $Y(\kappa)$ is implicitly defined by[3,4]

$$1 - (1 - \bar{u}) Y = \bar{u} \left[1 + \left(\frac{\Lambda}{\kappa}\right)^2\right]^{1/2} Y^{\nu/\Delta}. \tag{S20}$$

The function $Y$ has an asymptotic limit of $Y \to (\kappa/\bar{u}\Lambda)^{\Delta/\nu}$ for $\kappa \to 0$ and a limit of 1 for $\kappa \gg 1$, thus providing a smooth crossover to the mean-field equation of state (S1) far away from the critical point. To make the crossover function more explicit, we simplify equation (S20) by adopting $\bar{u} = 1$,[11]

$$Y(\kappa) = \left(1 + \frac{\Lambda^2}{\kappa^2}\right)^{-\Delta/(2\nu)}.$$

In this case, the crossover function is characterized by a single parameter $\Lambda$, which is related to the Ginzburg number $N_{\mathrm{G}}$ by[3]

$$N_{\mathrm{G}} = \frac{n_0 \Lambda^2}{c_t},$$

where the universal number $n_0 \simeq 0.0314$.[3] We also adopt $\bar{u}\Lambda = 0.5$, which is typical for near-critical fluids,[8] thus $\Lambda = 0.5$, giving $c_\rho \simeq 2$. The effective distance from the critical point $\kappa$, which is inversely proportional to the correlation length of the order-parameter fluctuations,[3,8] can be calculated from the mean-field value $\kappa_{\mathrm{mf}}$ with the relation[12–14]

$$\kappa^2 = \frac{Y^{\nu/(2\Delta)}}{c_\rho^2} \kappa_{\mathrm{mf}}^2 (x_\times, \Delta \hat{P}_\times),$$

where the mean-field distance $\kappa_{\mathrm{mf}}$ is evaluated at the renormalized concentration $x_\times$ and pressure $\Delta \hat{P}_\times$. The mean-field distance is related to the mean-field strong susceptibility $\chi_{1,\mathrm{mf}}$ according to

$$\kappa_{\mathrm{mf}}^2 = \chi_{1,\mathrm{mf}}^{-1}.$$

With the expression for $\chi_{1,\mathrm{mf}}$ [equation (S11)], we obtain

$$\kappa^2 = \frac{Y^{\nu/(2\Delta)}}{c_\rho^2} \left[\frac{1}{2 x_\times (1 - x_\times)} - \omega(\Delta \hat{P}_\times)\right]. \tag{S21}$$

Together with equation (S19), the condition for chemical reaction equilibrium, $(\partial \hat{G}_\times / \partial x)_{\hat{P}, \hat{T}} = 0$, yields the condition for the equilibrium concentration $x = x_{\mathrm{e}}$,

$$\begin{aligned} \ln K + \left(\frac{\partial x_\times}{\partial x}\right)_P \left[\ln\left(\frac{x_\times}{1 - x_\times}\right) + \omega(\Delta \hat{P}_\times)(1 - 2x_\times)\right] \\ - \left(x_\times - \frac{1}{2}\right)^2 \omega_0 \left(\frac{\partial \Delta \hat{P}_\times}{\partial x}\right)_P + \frac{1}{2} \left(\frac{\partial k}{\partial x}\right)_P = 0. \end{aligned} \tag{S22}$$

This equation is the crossover analogue of equation (3). The order parameter $\phi_1$, like in the mean-field approximation, is related to the concentration $x$ by

$$\phi_1 = \Delta\hat{x}.$$

Analogous to the mean-field case, the scaling densities and susceptibilities are found as derivatives of the potential $\Phi_\times$. The scaling density $\phi_2$ is

$$\begin{aligned}\phi_2 &= \left(\frac{\partial\Phi_\times}{\partial\hat{P}}\right)_x \\ &= 2\left(\frac{\partial x_\times}{\partial\hat{P}}\right)_x\left[\ln\left(\frac{x_\times}{1-x_\times}\right)+\omega(\Delta\hat{P}_\times)(1-2x_\times)\right] \\ &\quad + 2\left(\frac{\partial\Delta\hat{P}_\times}{\partial\hat{P}}\right)_x\omega_0\big[x_\times(1-x_\times)-1/4\big]+\left(\frac{\partial k}{\partial\hat{P}}\right)_x.\end{aligned}$$

The strong susceptibility $\chi_1$ is given by

$$\begin{aligned}\chi_1^{-1} &= \frac{1}{4}\left(\frac{\partial^2\Phi_\times}{\partial x^2}\right)_P \\ &= \frac{1}{2}\left\{\left(\frac{\partial^2 x_\times}{\partial x^2}\right)_P\ln\left(\frac{x_\times}{1-x_\times}\right)+\left(\frac{\partial x_\times}{\partial x}\right)_P^2\frac{1}{x_\times(1-x_\times)}\right. \\ &\quad - 2\omega(\Delta\hat{P}_\times)\left[\left(\frac{\partial x_\times}{\partial x}\right)_P^2+(x_\times-1/2)\left(\frac{\partial^2 x_\times}{\partial x^2}\right)_P\right] \\ &\quad - 4(x_\times-1/2)\left(\frac{\partial x_\times}{\partial x}\right)_P\omega_0\left(\frac{\partial\Delta\hat{P}_\times}{\partial x}\right)_P \\ &\quad \left. - (x_\times-1/2)^2\omega_0\left(\frac{\partial^2\Delta\hat{P}_\times}{\partial x^2}\right)_P\right\}+\frac{1}{4}\left(\frac{\partial^2 k}{\partial x^2}\right)_P.\end{aligned}$$

The cross susceptibility $\chi_{12}$ is given by

$$\begin{aligned}\chi_{12} &= \frac{1}{2}\left(\frac{\partial^2\Phi_\times}{\partial x\partial\hat{P}}\right)\chi_1 \\ &= \chi_1\left\{\frac{\partial^2 x_\times}{\partial x\partial\hat{P}}\left[\ln\left(\frac{x_\times}{1-x_\times}\right)-2(x_\times-1/2)\omega(\Delta\hat{P}_\times)\right]\right. \\ &\quad + \left(\frac{\partial x_\times}{\partial x}\right)_P\left(\frac{\partial x_\times}{\partial\hat{P}}\right)_x\left[\frac{1}{x_\times(1-x_\times)}-2\omega(\Delta\hat{P}_\times)\right] \\ &\quad - 2(x_\times-1/2)\omega_0\left[\left(\frac{\partial x_\times}{\partial x}\right)_P\left(\frac{\partial\Delta\hat{P}_\times}{\partial\hat{P}}\right)_x\right. \\ &\qquad \left. + \left(\frac{\partial x_\times}{\partial\hat{P}}\right)_x\left(\frac{\partial\Delta\hat{P}_\times}{\partial x}\right)_P\right] \\ &\quad \left. - (x_\times-1/2)^2\omega_0\frac{\partial^2\Delta\hat{P}_\times}{\partial x\partial\hat{P}}\right\}+\frac{1}{2}\frac{\partial^2 k}{\partial x\partial\hat{P}}.\end{aligned}$$

The weak susceptibility $\chi_2$ is given by

$$\begin{aligned}\chi_2 &= \frac{\chi_{12}^2}{\chi_1}-\left(\frac{\partial^2\Phi_\times}{\partial\hat{P}^2}\right)_x \\ &= \frac{\chi_{12}^2}{\chi_1}-2\left\{\left(\frac{\partial^2 x_\times}{\partial\hat{P}^2}\right)_x\left[\ln\left(\frac{x_\times}{1-x_\times}\right)+\omega(\Delta\hat{P}_\times)(1-2x_\times)\right]\right. \\ &\quad + \left(\frac{\partial x_\times}{\partial\hat{P}}\right)_x^2\left[\frac{1}{x_\times(1-x_\times)}-2\omega(\Delta\hat{P}_\times)\right] \\ &\quad - \left(\frac{\partial^2\Delta\hat{P}_\times}{\partial\hat{P}^2}\right)_x\omega_0(x_\times-1/2)^2 \\ &\quad \left. + 2\omega_0\left(\frac{\partial\Delta\hat{P}_\times}{\partial\hat{P}}\right)_x(1-2x_\times)\left(\frac{\partial x_\times}{\partial\hat{P}}\right)_x\right\}-\left(\frac{\partial^2 k}{\partial\hat{P}^2}\right)_x.\end{aligned}$$

The procedure to calculate the properties at a certain temperature and pressure is as follows. First, the equilibrium fraction $x_e$ and the distance $\kappa$ are calculated by solving the set of equations (S21) and (S22). Then, the scaling densities and susceptibilities are computed using the equations in this section. Finally, the properties are calculated from equations (S7) and (S8).

## 4. FIT TO EXPERIMENTAL DATA

### A. Ordinary water

The LLT curve in the $P$–$T$ plane is represented by the curve $\ln K = 0$. Because the LLT curve is located in the experimentally inaccessible region, there is only indirect experimental evidence of its location. Mishima measured metastable melting curves of $H_2O$ ice IV[15] and $D_2O$ ices IV and V,[16] and found that they suddenly bent at temperatures of 4 K to 7 K below $T_H$, which suggests that the ice melts to a different liquid phase there. Kanno and Angell[17] fitted empirical power laws to their compressibility measurements and found that the temperatures of apparent divergences of the compressibility were located 5 K to 12 K below the homogeneous nucleation curve. The curve of temperatures of divergence of Kanno and Angell and Mishima's LLT curve[18] are similar; they have the same shape as the homogeneous nucleation curve but are shifted to lower temperature and pressure. A simple equation that fairly reproduces the shape of the homogeneous nucleation curve is a hyperbola. At low temperature, this curve becomes relatively flat in the $P$–$T$ diagram, which is necessary for a connection with the amorphous LDA/HDA transition. To satisfy this feature, we adopt the equilibrium constant as

$$\ln K = \lambda(\Delta\hat{T}+a\Delta\hat{P}+b\Delta\hat{T}\Delta\hat{P}).$$

Here $a = -\mathrm{d}\hat{T}/\mathrm{d}\hat{P}$ is the slope of the LLT curve ($\ln K = 0$) at the critical point, and $b$ determines the curvature.

For $H_2O$, the data set to which the equation of state was fitted covers the range of 140 K to 310 K and 0.1 MPa to 400 MPa, contains 252 points, and contains data for the density, isothermal compressibility, thermal expansion coefficient, isobaric heat capacity, and speed of sound. The data

TABLE S1. Parameters for the crossover equation of state for $H_2O$

| Parameter | Value | Parameter | Value |
|---|---|---|---|
| $T_c$/K | 227.42 | $c_{05}$ | $2.1652 \times 10^{-5}$ |
| $P_c$/MPa | 13.45 | $c_{11}$ | $1.7738 \times 10^{-1}$ |
| $\rho_c$/(kg m$^{-3}$) | 928.46 | $c_{12}$ | $-2.1032 \times 10^{-2}$ |
| $\lambda$ | 2.3096 | $c_{13}$ | $2.1660 \times 10^{-3}$ |
| $\omega_0$ | 0.35253 | $c_{20}$ | $-3.9228 \times 10^{0}$ |
| $N_G$ | 0.092 | $c_{21}$ | $1.1495 \times 10^{-2}$ |
| $a$ | 0.065306 | $c_{22}$ | $-8.4263 \times 10^{-3}$ |
| $b$ | −0.28051 | $c_{23}$ | $-9.5657 \times 10^{-4}$ |
| $c_{02}$ | $-8.1577 \times 10^{-3}$ | $c_{30}$ | $7.0848 \times 10^{-1}$ |
| $c_{03}$ | $1.0969 \times 10^{-3}$ | $c_{31}$ | $2.0613 \times 10^{-3}$ |
| $c_{04}$ | $-2.6244 \times 10^{-4}$ | $c_{32}$ | $2.0217 \times 10^{-2}$ |

TABLE S2. Parameters for the crossover equation of state for $D_2O$

| Parameter | Value | Parameter | Value |
|---|---|---|---|
| $T_c$/K | 232.25 | $c_{05}$ | $-8.9099 \times 10^{-6}$ |
| $P_c$/MPa | 13.36 | $c_{11}$ | $1.9287 \times 10^{-1}$ |
| $\rho_c$/(kg m$^{-3}$) | 1004.0 | $c_{12}$ | $-8.2222 \times 10^{-3}$ |
| $\lambda$ | 3.1505 | $c_{13}$ | $-2.1506 \times 10^{-3}$ |
| $\omega_0$ | 0.32959 | $c_{20}$ | $-4.2149 \times 10^{0}$ |
| $N_G$ | 0.098 | $c_{21}$ | $1.3640 \times 10^{-2}$ |
| $a$ | 0.0580 | $c_{22}$ | $-4.9486 \times 10^{-2}$ |
| $b$ | −0.2742 | $c_{23}$ | $4.7677 \times 10^{-3}$ |
| $c_{02}$ | $-1.2294 \times 10^{-2}$ | $c_{30}$ | $6.9872 \times 10^{-1}$ |
| $c_{03}$ | $1.8962 \times 10^{-3}$ | $c_{31}$ | $-9.7268 \times 10^{-2}$ |
| $c_{04}$ | $-1.5045 \times 10^{-4}$ | $c_{32}$ | $8.9969 \times 10^{-2}$ |

set is identical to the 'extended-range' data set discussed in Ref. 19, except for the following differences. In the current set we have included densities of low-density and high-density amorphous ice,[20] because we assume that the liquid–liquid phase transition is connected to the amorphous–amorphous phase transition that exists below about 140 K. Second, we have fitted the model to heat-capacity data of Angell *et al.*[21] instead of Archer and Carter,[22] because the deviations from data for the heat capacity, expansivity, and density were lower when the data of Angell *et al.* were used.

We have fitted both the mean-field and the crossover equation of state to the experimental data. For the mean-field equation of state, the optimum locations of the critical point form a narrow band in the $P$–$T$ diagram, which extends approximately from 222 K and −50 MPa to 240 K and 30 MPa. The most likely location of the LLT curve, as follows from the suggestions of Mishima[16] and Kanno and Angell,[17] intersects the band of optimum critical point locations at about zero pressure; see Fig. S2(a). For the crossover equation of state, the region of possible critical point locations is similar to that of the mean-field model, but shifted by about 10 MPa to higher pressures, as shown in Fig. S2(b). The best fit for the critical point is obtained at about 227 K and 13.5 MPa; a list of all parameter values is given in Table S1. It is not surprising that the fit of the mean-field version of our equation of state has the same quality as the fit of the crossover version, because the experimental data are located beyond the region strongly affected by fluctuations ($h_1, h_2 \ll N_G \sim 0.1$, typical for a liquid–liquid transition[24]).

### B. Heavy water

For $D_2O$, the data set covers the range of 240 K to 305 K and 0.1 MPa to 150 MPa, and contains 169 points, as described in Ref. 19. The fit of the crossover equation of state yields a region of critical point locations that is broader than for $H_2O$, which is the result of a lack of accurate data for the density of low-density and high-density amorphous $D_2O$. The location of the critical point was constrained by using the principle of corresponding states, that is, the critical compressibility factor

$$Z_c = \frac{P_c v_c}{k_B T_c} \tag{S23}$$

where $v_c$ is the critical molecular volume, should be the same for $H_2O$ and $D_2O$. With this constraint, the optimum critical point was found at 232 K and 13.4 MPa; see Table S2. The density and response functions are shown in Figs. S3 and S4.

## 5. HEAT CAPACITY BELOW THE CRITICAL TEMPERATURE

As Fig. 4b shows, the predicted isobaric and isochoric heat capacities $C_P$ and $C_V$ show strong asymmetry around their maxima. The source of this asymmetry is the term proportional to $\phi_1 + 1 = 2x$ in equation (S8). In our equation of state, the temperature dependence of the fraction $x$ is exactly antisymmetric (Fig. 6), which results in the large asymmetry of the heat capacity. Without the contribution from the $2x$ term, the heat capacity would be almost symmetric, as the dotted line in Fig. 4b shows. The only source of asymmetry in this case is the noncritical background. The experimental data on the heat capacity of confined water[32] suggest that some asymmetry may be present, but not as much as our equation of state predicts. If needed, the degree of asymmetry can be easily changed by adding a cubic term with respect to $x$ in the non-ideal part of equation (S1).

## 6. FRACTION OF THE LOW-DENSITY STATE

In Fig. 6 of the main article, we compare the fraction $x$ in the two-state model with the fraction $f$ of four-coordinated molecules in the simulations of the mW model performed by Moore and Molinero.[33] In the mW simulations, the fraction $f$ does not vanish at room temperature since the pure high-density liquid is a mixture of four-coordinated and higher-coordinated molecules. In the low-density liquid, on the other hand, nearly all molecules are four-coordinated. To convert $f$ to $x$, we assume that the fractions $x$ and $f$ are related by

$$f = x f_{LDL} + (1 - x) f_{HDL}, \tag{S24}$$

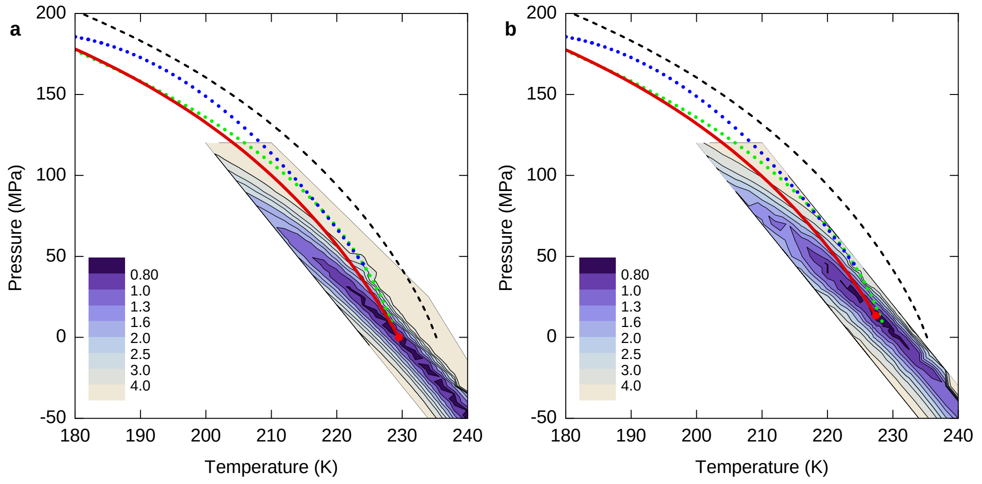


FIG. S2. **Optimization of the LLCP location.** **a**, Mean-field equation of state, **b**, Crossover equation of state. The coloured map shows the reduced sum of squared residuals. The solid red line is the hypothesized LLT curve. The dashed curve shows the temperature of homogeneous ice nucleation.[23] The blue dotted curve is the LLT suggestion by Mishima[18] and the green dotted curve is the 'singularity' line suggested by Kanno and Angell.[17]

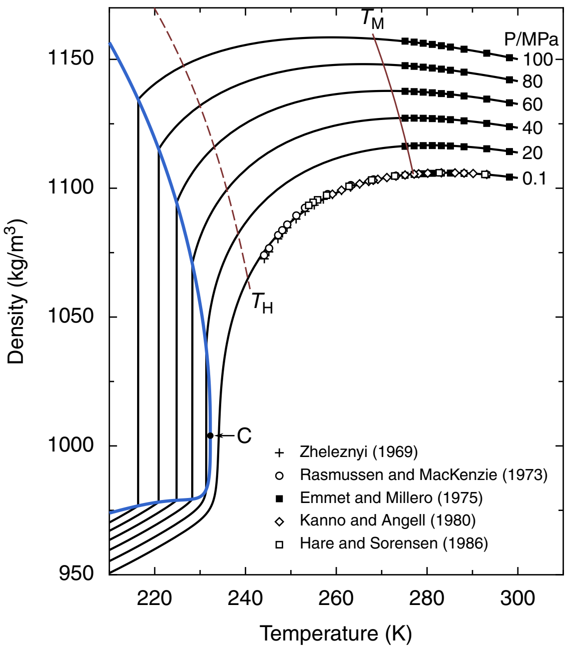


FIG. S3. **Density of cold and supercooled $D_2O$ as a function of temperature and pressure.** Black curves are the predictions of the crossover two-state model. $T_M$ (thin black) indicates the melting temperature[25] and $T_H$ indicates the homogeneous nucleation temperature.[26] The thin blue line is the liquid–liquid equilibrium curve, with the critical point C. Symbols represent experimental data.[27–31]

where $f_{LDL} \simeq 1$. For $f_{HDL} = 0.2$, the high-temperature tail of the mW fraction $x$ is close to the fraction $x$ in the two state model, as shown in Fig. S5. As noted in Ref. 33, the sigmoid-like form of $x$ points to strong cooperativity for both real water and the mW model that evidences the strong non-ideality which eventually leads to phase separation, real or virtual.

## REFERENCES


1. Bertrand, C. E. & Anisimov, M. A. The peculiar thermodynamics of the second critical point in supercooled water. *J. Phys. Chem. B* **115**, 14099–14111 (2011).
2. Fisher, M. E. Scaling, universality and renormalization group theory. In Hahne, F. J. W. (ed.) *Critical Phenomena, Lecture Notes in Physics*, vol. 186, 1–139 (Springer, Berlin, 1983).
3. Anisimov, M. A. & Sengers, J. V. Critical region. In Sengers, J. V., Kayser, R. F., Peters, C. J. & White, H. J., Jr. (eds.) *Equations of State for Fluids and Fluid Mixtures*, vol. V of *Experimental Thermodynamics*, chap. 11, 381–434 (Elsevier, Amsterdam, 2000).
4. Behnejad, H., Sengers, J. V. & Anisimov, M. A. Thermodynamic behavior of fluids near critical points. In Goodwin, A. R. H., Sengers, J. V. & Peters, C. J. (eds.) *Applied Thermodynamics of Fluids*, chap. 10, 321–367 (RSC Publishing, Cambridge, UK, 2010).
5. Landau, L. D. & Lifshitz, E. M. *Statistical Physics*, vol. 5 of *Course of Theoretical Physics* (Pergamon, Oxford, 1980), 3 edn.
6. Debenedetti, P. G. Supercooled and glassy water. *J. Phys.: Condens. Matter* **15**, R1669–R1726 (2003).
7. Fisher, M. E. & Zinn, S.-Y. The shape of the van der Waals loop and universal critical amplitude ratios. *J. Phys. A* **31**, L629–L635 (1998).
8. Anisimov, M. A., Kiselev, S. B., Sengers, J. V. & Tang, S. Crossover approach to global critical phenomena in fluids. *Physica A* **188**, 487–525 (1992).
9. Pelissetto, A. & Vicari, E. Critical phenomena and renormalization-group theory. *Phys. Rep.* **368**, 549–727 (2002).
10. Sengers, J. V. & Shanks, J. G. Experimental critical-exponent values for fluids. *J. Stat. Phys.* **137**, 857–877 (2009).

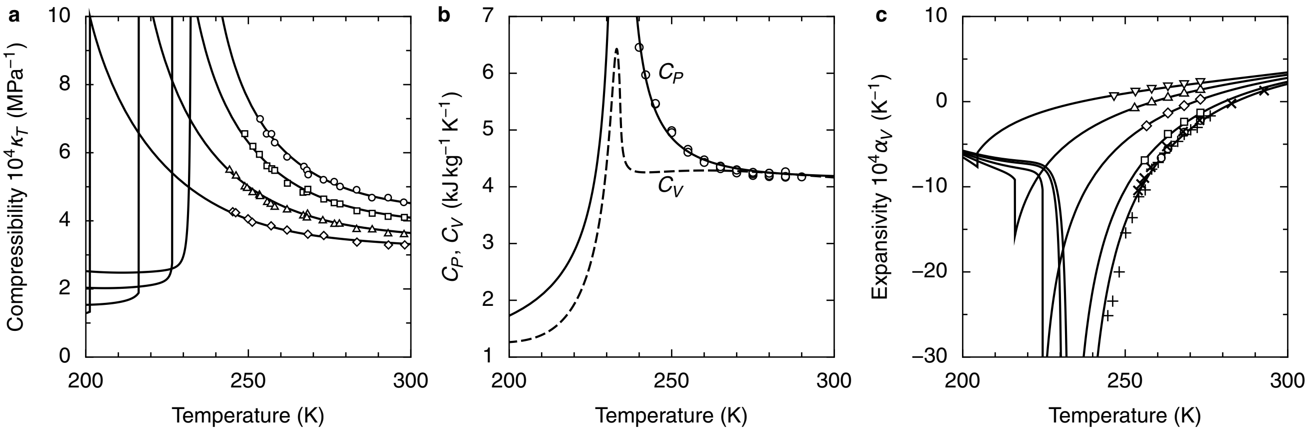


FIG. S4. **Response functions of $D_2O$ as a function of temperature.** **a**, Isothermal compressibility.[17] Pressures, from top to bottom: 10 MPa, 50 MPa, 100 MPa, 150 MPa. **b**, Heat capacity at constant pressure[21] $C_P$ and at constant volume $C_V$ (calculated) at 0.1 MPa. **c**, Thermal expansivity.[27,30,31] Pressures, from top to bottom: 140 MPa, 100 MPa, 60 MPa, 20 MPa, 0.1 MPa. In **a, b,** and **c,** the curves are the prediction of the crossover two-state model, and the symbols represent experimental data.

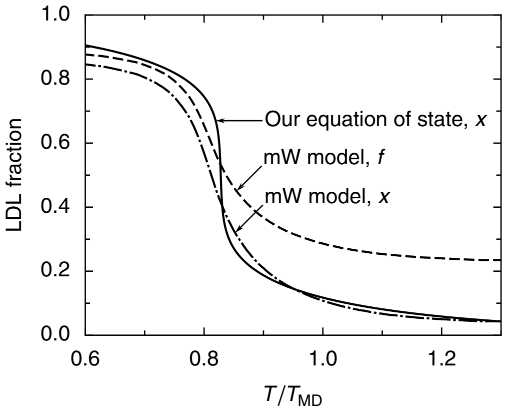


FIG. S5. **Fraction of molecules in the low-density state.** The fraction $x$ is shown for the two-state crossover model at 0.1 MPa, and for mW water simulations performed by Moore and Molinero.[33] The fraction $x$ for the mW model (dashed-dotted) is calculated from the fraction of four-coordinated molecules $f$ (dashed) according to equation (S24). The temperature is scaled by the temperature of maximum density $T_{\mathrm{MD}}$ (250 K for the mW model and 277 K for real water).


[11] Anisimov, M. A., Kostko, A. F. & Sengers, J. V. Competition of mesoscales and crossover to tricriticality in polymer solutions. *Phys. Rev. E* **65**, 051805 (2002).

[12] Edison, T. A., Anisimov, M. A. & Sengers, J. V. Critical scaling laws and an excess Gibbs energy model. *Fluid Phase Equilib.* **150–151**, 429–438 (1998).

[13] Povodyrev, A. A., Anisimov, M. A. & Sengers, J. V. Crossover Flory model for phase separation in polymer solutions. *Physica A* **264**, 345–369 (1999).

[14] van 't Hof, A., Japas, M. L. & Peters, C. J. Description of liquid–liquid equilibria including the critical region with the crossover-NRTL model. *Fluid Phase Equilib.* **192**, 27–48 (2001).

[15] Mishima, O. & Stanley, H. E. Decompression-induced melting of ice IV and the liquid–liquid transition in water. *Nature* **392**, 164–168 (1998).

[16] Mishima, O. Liquid-liquid critical point in heavy water. *Phys. Rev. Lett.* **85**, 334–336 (2000).

[17] Kanno, H. & Angell, C. A. Water: Anomalous compressibilities to 1.9 kbar and correlation with supercooling limits. *J. Chem. Phys.* **70**, 4008–4016 (1979).

[18] Mishima, O. Volume of supercooled water under pressure and the liquid-liquid critical point. *J. Chem. Phys.* **133**, 144503 (2010).

[19] Holten, V., Bertrand, C. E., Anisimov, M. A. & Sengers, J. V. Thermodynamics of supercooled water. *J. Chem. Phys.* **136**, 094507 (2012).

[20] Loerting, T. *et al.* How many amorphous ices are there? *Phys. Chem. Chem. Phys.* **13**, 8783–8794 (2011).

[21] Angell, C. A., Oguni, M. & Sichina, W. J. Heat capacity of water at extremes of supercooling and superheating. *J. Phys. Chem.* **86**, 998–1002 (1982).

[22] Archer, D. G. & Carter, R. W. Thermodynamic properties of the NaCl + $H_2O$ system. 4. Heat capacities of $H_2O$ and NaCl(aq) in cold-stable and supercooled states. *J. Phys. Chem. B* **104**, 8563–8584 (2000).

[23] Kanno, H. & Miyata, K. The location of the second critical point of water. *Chem. Phys. Lett.* **422**, 507–512 (2006).

[24] Anisimov, M. A., Povodyrev, A. A., Kulikov, V. D. & Sengers, J. Nature of crossover between Ising-like and mean-field critical behavior in fluids and fluid mixtures. *Phys. Rev. Lett.* **75**, 3146–3149 (1995).

[25] Bridgman, P. W. The pressure-volume-temperature relations of the liquid, and the phase diagram of heavy water. *J. Chem. Phys.* **3**, 597–605 (1935).

[26] Angell, C. A. & Kanno, H. Density maxima in high-pressure supercooled water and liquid silicon dioxide. *Science* **193**, 1121–1122 (1976).

[27] Zheleznyi, B. V. The density of supercooled water. *Russ. J. Phys. Chem.* **43**, 1311 (1969).

[28] Rasmussen, D. H. & MacKenzie, A. P. Clustering in supercooled water. *J. Chem. Phys.* **59**, 5003–5013 (1973).

[29] Emmet, R. T. & Millero, F. J. Specific volume of deuterium

oxide from 2° to 40°C and 0 to 1000 bars applied pressure. *J. Chem. Eng. Data* **20**, 351–356 (1975).

[30] Kanno, H. & Angell, C. A. Volumetric and derived thermal characteristics of liquid $D_2O$ at low temperatures and high pressures. *J. Chem. Phys.* **73**, 1940–1947 (1980).

[31] Hare, D. E. & Sorensen, C. M. Densities of supercooled $H_2O$ and $D_2O$ in 25 μ glass capillaries. *J. Chem. Phys.* **84**, 5085–5089 (1986).

[32] Nagoe, A., Kanke, Y., Oguni, M. & Namba, S. Findings of $C_p$ maximum at 233 K for the water within silica nanopores and very weak dependence of the $T_{\max}$ on the pore size. *J. Phys. Chem. B* **114**, 13940–13943 (2010).

[33] Moore, E. B. & Molinero, V. Growing correlation length in supercooled water. *J. Chem. Phys.* **130**, 244505 (2009).
